# Supplementary material for: A Message Passing based Adaptive PDA Algorithm for Robust Radio-based Localization and Tracking
Source: arXiv:2103.13188 source file (2021-03-25)
Supplement: Supplementary file 1 [file appendix.tex]

% placeholder for appendix
% dont think there will be one
% maybe further work?
